# Supplementary material for: Simons Lectures on Categorical Symmetries
Source: arXiv:2411.09082 source file (2024-11-13)
Supplement: Supplementary file 1 [file main.tex]

\setcounter{section}{0}
    \setcounter{example}{0}
    \setcounter{figure}{0}

    \phantomsection
    \addcontentsline{toc}{section}{{\large Appendix: quick guide to the literature}\\
    \texorpdfstring{\textnormal{\textit{Covers papers published till \today}}\vspace{-0.2cm}}{}
    }

    \begin{center}
        {\LARGE {\bf Appendix: quick guide to the literature}}\\

        \vspace{0.2cm}
        
        ---
        
        \textit{Covers papers published till \today}
    \end{center}

\textbf{[XXXMDZ: THIS IS VERY LIKELY NEVER GOING TO HAPPEN, RIGHT????]}

\section{Generalized Global Symmetries}

\section{Higher groups}

\section{Non-Invertible Symmetries}

\section{Extended Topological Field Theories}

\section{n-Fusion Categories}
